# Supplementary material for: Learning Co-Speech Gesture Representations in Dialogue through Contrastive Learning: An Intrinsic Evaluation
Source: arXiv:2409.10535 source file (2024-08-31)
Supplement: Supplementary file 1 [file additional_results.tex]

\begin{figure*}[!h]
    \centering
    \begin{subfloat}[SLR baseline model]{
        \includegraphics[width=0.32\linewidth]{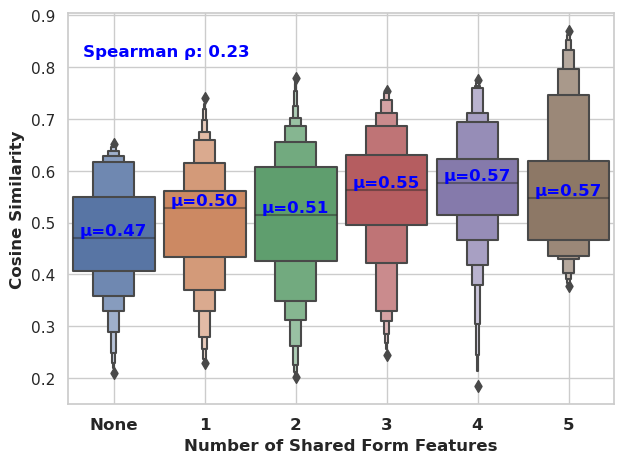}}
        \label{fig:slr_box}
    \end{subfloat}
    \begin{subfloat}[Unimodal contrastive model]{
        \includegraphics[width=0.32\linewidth]{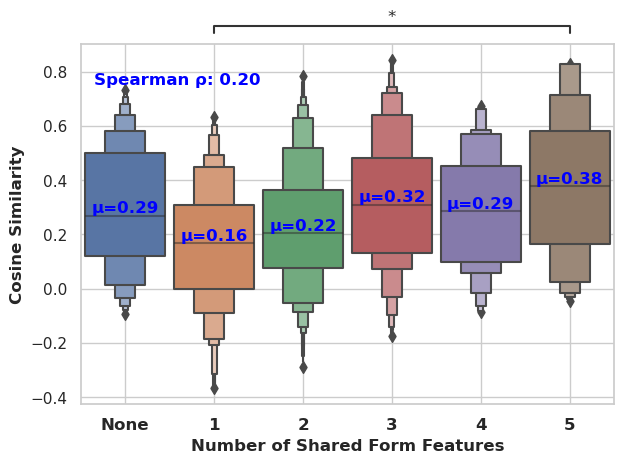}}
    \end{subfloat}
    \begin{subfloat}[Multimodal model]{
        \includegraphics[width=0.32\linewidth]{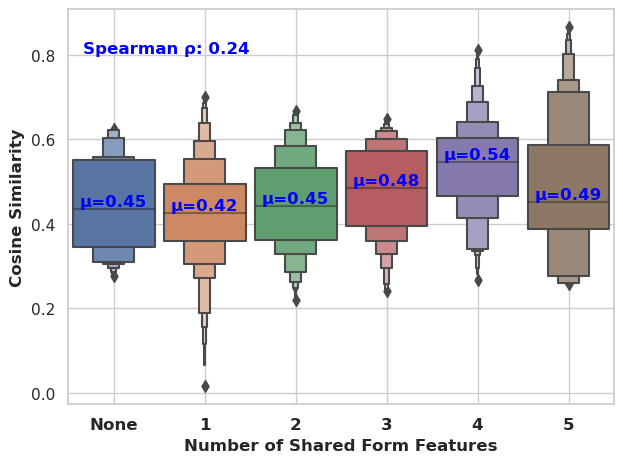}}
        \label{fig:mm_box}
    \end{subfloat}
    \Description[]{}
\caption{Distribution of cosine similarities between gesture pairs with different numbers of shared form features.}
\label{fig:baseline_similarities}
\end{figure*}

\label{sect:additional_results}
\subsection{Evaluation of Model Representations}
Section 5 presents an intrinsic evaluation of model representations using a set of gesture pairs with manually annotated similarity in terms of form features. In this appendix, we complement this analysis with cosine similarity score distributions for the remaining models. Figure \ref{fig:baseline_similarities} demonstrates these distributions for the \textbf{SLR baseline}, and models trained with \textbf{unimodal} (Section 4.2) and \textbf{multimodal} (Section 4.3) contrastive objectives.

Section 5.1 reports that the combined objective model produces the highest Spearman correlation, followed by multimodal, SLR, and unimodal models.
Additionally, the model trained with the combined objective (as shown in Figure 4) produces the highest absolute differences of 0.27 between the average similarity scores of pairs that are annotated as the most similar (with 5 shared features) and pairs that are not similar in any dimension. However, this absolute difference is lower for the other models. Furthermore, all the baselines show high similarity scores even when expert annotations do not indicate any similarities between gestures. Finally, according to the conducted statistical tests, significant differences are obtained only after unimodal training between similarity distributions with 1 and 5 shared form features.

\subsection{Gesture Similarity in Referential Dialogues}

\subsubsection{Referent vs.~Speaker Driven Similarity}
\label{sect:dialogue_based_analysis_appendix}
In section 5.2.1, we find that the multimodal representations trained with the combined objective comply with the two hypotheses: 

\begin{itemize}[leftmargin=24pt,itemsep=3pt]
\item[H1 a.] Representations of gestures by the same speaker will be more similar if the gestures have the same referent than if they refer to different objects.
\item[\ \ \ b.] Representations of gestures made by different speakers will be more similar if the gestures have the same referent than if they refer to different objects.
\item[H2 \; ] Representations of gestures with the same referent will be more similar if the gestures are produced by the same speaker than if they are made by different speakers.
\end{itemize}

The results for the SLR baseline and the models trained with unimodal and multimodal contrastive objectives are shown in Figure \ref{fig:baselines_voilin}. All models comply with the two hypotheses. However, the models trained solely on skeleton data (i.e., SLR and Unimodal models) did not show any significant differences in the similarity between the sets of same-referent-different-speaker and different-referent-same-speaker.
We believe that adding speech to models trained with multimodal and combined objectives might have resulted in representations that could amplify individuals' unique voice and speech characteristics, independent of the referent.

It is worth noting that the cosine similarity scale varies across the three models. For example, the SLR and multimodal models have a higher average score, while the unimodal model has a lower score. The unimodal model's low scores are due to the contrastive objective applied to skeleton data. This objective leads to a lower similarity score between gesture pairs since the objective aims to minimize the distances between different views of the same gesture and maximize the distances between different gesture pairs. On the other hand, the multimodal model is not trained with the same objective as the contrastive learning applied cross-modally, resulting in higher similarity scores between gesture pairs' representations, as in the original SLR model.

\begin{figure*}[!h]
    \centering
    \begin{subfloat}[SLR baseline]{
        \includegraphics[width=0.32\linewidth]{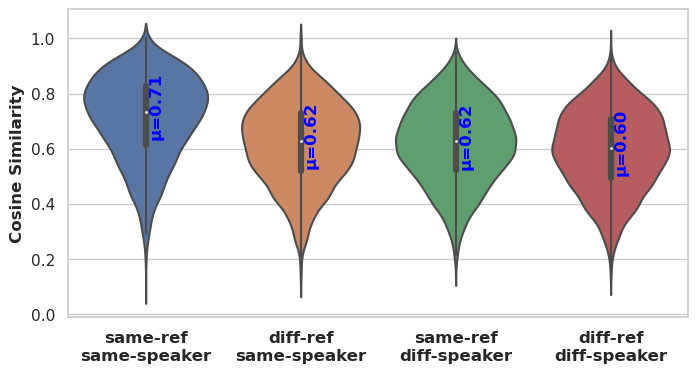}}
        \label{fig:slr_violin}
    \end{subfloat}
    \begin{subfloat}[Unimodal contrastive objective]{
        \includegraphics[width=0.32\linewidth]{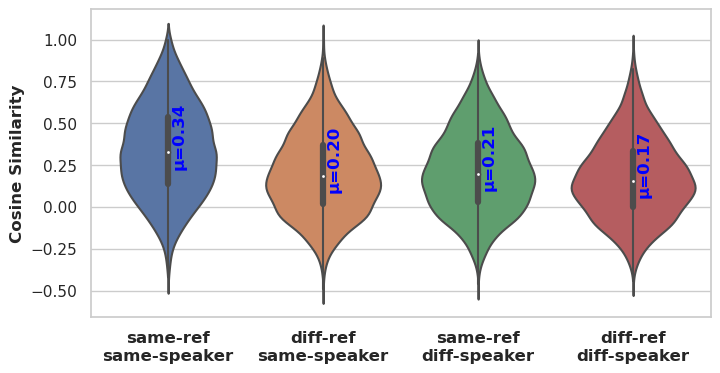}}
        \label{fig:unimodal_violin}
    \end{subfloat}
    \begin{subfloat}[Cross-modal objective]{
        \includegraphics[width=0.32\linewidth]{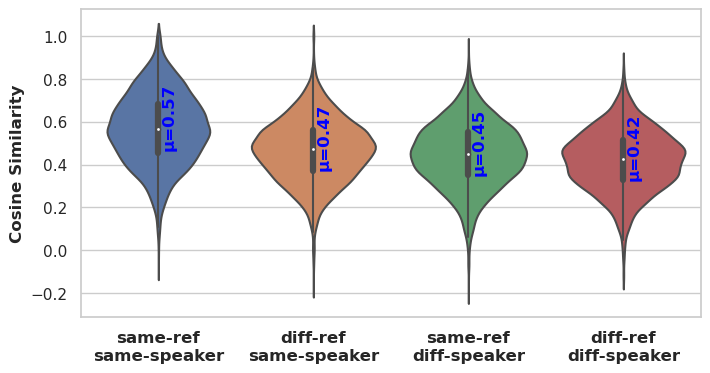}}
        \label{fig:violin_mm}
    \end{subfloat}
    \Description[]{}
\caption{Distribution of cosine similarity scores of self and across-speaker gesture pairs in a dialogue when referring to the same or different referents. The labels `same-ref' / `diff-ref' indicate whether the gestures in a pair refer to the same object or not. Based on the independent t-test with Bonferroni correction, the similarity score distributions in all sets are significantly different except for two cases. Specifically, for both the SLR and Unimodal models, the similarity between the sets of same-referent-different-speaker and different-referent-same-speaker did not differ significantly.}
\label{fig:baselines_voilin}
\end{figure*}

\subsubsection{Referent vs.~Interaction Driven Similarity}\
In section 5.2.2, we formulate the following hypothesis:

\begin{itemize}[leftmargin=20pt]
    \item[H3 \ ] Representations of gestures by different speakers will be more similar when the two speakers are interlocutors within a dialogue than when the speakers are from different dialogues.
\end{itemize}

We note that the multimodal representations resulting from the model trained with the combined objective comply with H3. The results for the remaining models are presented in Figure \ref{fig:baseline_bars}, where it can be seen that all the models' representations also fulfill H3.

\begin{figure*}[h]
    \centering
    \begin{subfloat}[SLR baseline]{
        \includegraphics[width=0.32\linewidth]{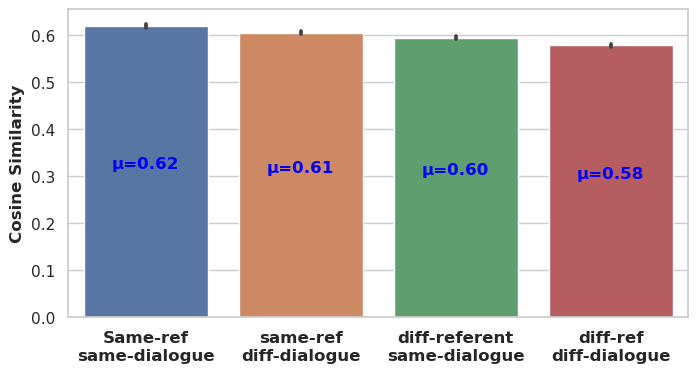}}
        \label{fig:slr_bar}
    \end{subfloat}
    \begin{subfloat}[Unimodal contrastive model]{
        \includegraphics[width=0.32\linewidth]{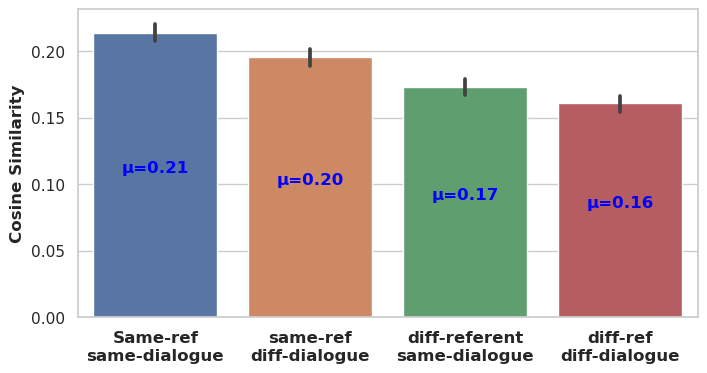}}
         \label{fig:bar_unimodal}
    \end{subfloat}
    \begin{subfloat}[Cross-modal model]{
        \includegraphics[width=0.32\linewidth]{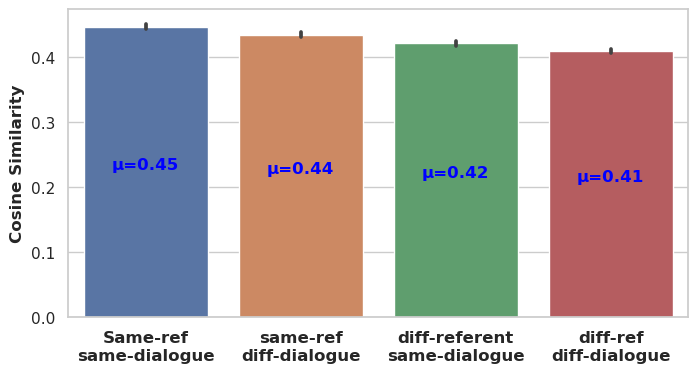}}
        \label{fig:bar_mm}
    \end{subfloat}
    \Description[]{}
\caption{Similarity scores of gesture representation pairs by different speakers. The labels `same-ref' / `diff-ref' indicate whether the gestures in a pair refer to the same object or not; the labels `same-dialogue' / `diff-dialogue' indicate whether the speakers are interlocutors within the same dialogue or are participants from different dialogues. Independent t-test with Bonferroni correction shows that all sets' distributions of similarity scores are significantly different from each other.}
\label{fig:baseline_bars}
\end{figure*}
