# Supplementary material for: Learning Co-Speech Gesture Representations in Dialogue through Contrastive Learning: An Intrinsic Evaluation
Source: arXiv:2409.10535 source file (2024-08-31)
Supplement: Supplementary file 2 [file dataset.tex]

\subsection{Manually Coded Gesture Form Similarity}
Rasenberg \etal~\cite{rasenberg2022primacy} report reasonable inter-annotator agreement for their gesture-pair similarity coding. The authors used 103 gesture pairs to study inter-annotator agreement for hand shape, orientation, movement, and position. Coders determined handedness using existing gesture annotations separated into left and right-hand tiers in ELAN (an annotation tool for audio and video recordings). As a result, the handedness agreement was part of the inter-rater agreement for gesture coding based on 264 gestures.

\begin{table}
    \centering
        \begin{tabular}{lcc}
            \toprule
            \textbf{Feature} & \textbf{0} & \textbf{1} \\
            \midrule
            Handedness & 196 & 223 \\
            Position   & 90  & 329 \\
            Shape      & 290 & 129 \\
            Movement   & 326 & 93  \\
            Rotation   & 253 & 166 \\
            \bottomrule
        \end{tabular}
        \captionof{table}{Distribution of values for each form feature.}
    \label{tab:distribution_of_binary_feats}
\end{table}

Handedness annotations showed a high
Cohen's kappa score (.91), with shape, movement, and orientation showing substantial to moderate agreement (kappa scores of .71, .63, .54, respectively). The lowest agreement was achieved for position, with a kappa score of .47. Table  \ref{tab:distribution_of_binary_feats} shows the distribution of the binary values per form feature for the 419 gesture pairs coded for similarity by the authors.
