# Supplementary material for: Learning Co-Speech Gesture Representations in Dialogue through Contrastive Learning: An Intrinsic Evaluation
Source: arXiv:2409.10535 source file (2024-08-31)
Supplement: Supplementary file 3 [file implementation_details.tex]

\subsection{Trainig Procedures and Hyperparameters}
We implement our models using Pytorch \cite{Ansel_PyTorch_2_Faster_2024} and the Pytorch-Lightning \cite{Falcon_PyTorch_Lightning_2019} framework. The experiments are conducted on a computational node with 2 NVIDIA RTX A5000 GPUs. The models are trained within the contrastive learning objectives for a maximum of 200 epochs using the Adam optimizer with a learning rate equal to 0.001. We find a batch size of 128 (per GPU) optimal for our experimentation, as the models can fit GPUs (with memory of 24 GB) and for the models' convergence. For the contrastive learning objective, we use a default temperature of 0.1. In model development, we use $90\%$ of the dataset (i.e., 63137-time windows) for training and $10\%$ for validation (i.e., 7016-time windows).

\subsection{Skeletal Augmentations}
The following is a list of the employed augmentations. 
\begin{itemize}
    \item \textbf{Mirror Poses:} Flips the pose across the vertical axis.
    \item \textbf{Shift Poses:} Translates each of the 27 joints in a pose randomly within a range from -30 to 30 units.
    \item \textbf{Scale Poses:} Scales the entire pose by a random factor between 0.5 and 1.5, altering the size of the pose while maintaining its shape.
    \item \textbf{Random Move:} Moves the pose based on a combination of random rotations (between -10 to 10 degrees), scaling (between 0.9 to 1.1), and translations (between -0.2 to 0.2 units) over a duration of 1 or 2-time units. 
    \item \textbf{Jittering:} Adds Gaussian noise with a standard deviation of 0.1 to each joint's position, creating slight variations in pose configuration.
    \item \textbf{Scaling:} Non-uniformly scales the pose x and y coordinates by a factor between 0.7 and 1.2. 
    \item \textbf{Rotation:} Rotates the pose around a specified anchor joint within a range of -15 to 15 degrees in steps of 2 degrees. 
    \item \textbf{Shear:} Applies a shearing transformation with a coefficient of 0.2 along the x and y coordinates, altering the geometry of the pose. 
\end{itemize}

We do not apply any audio augmentation for the speech waveforms. The implementation will be made available upon the acceptance of the paper.
